# Supplementary material for: Does the boson peak survive in an ultrathin oxide glass?
Source: arXiv:1907.12200 ancillary file (2019-07-29)
Supplement: Supplementary file 1 [file Supplemental.pdf]

# Supplemental information

D. L. Cortie,[1,*] M. J. Cyster,[2] J. S. Smith,[2] G. N. Iles,[3]
R. A. Mole,[4] N. de Souza,[4] D. Yu,[4] and J. H. Cole[2,†]

[1] *The Institute for Superconducting and Electronic Materials, University of Wollongong*

[2] *Chemical and Quantum Physics, School of Science, RMIT University, Melbourne, Victoria 3000, Australia*

[3] *Space Physics, School of Science, RMIT University, Melbourne, Victoria 3000, Australia*

[4] *The Australian Nuclear Science and Technology Organisation*

(Dated: 26 July, 2019)

* dcortie@uow.edu.au

† jared.cole@rmit.edu.au

## I. MOLECULAR DYNAMICS

In each simulation, a time step of 1.0 fs was used, with an initial equilibration period of 5.0 ps, before collecting the data. The temperature of the simulation was maintained via the Nose-Hoover thermostat[2, 3]. Production runs were run for 20-50 ps. Results were visualised and rendered using Visual Molecular Dynamics [4].The trajectories were then analysed with NMoldyn [5] in order to calculate the neutron scattering properties. The static structure factor S(Q) of the amorphous cells, weighted by the neutron coherent cross-section, was calculated and verified against experimental neutron data [1] in Figure 1. To calculate the dynamic scattering function, the intermediate real-time scattering function was calculated. This was then Fourier transformed, weighted by the coherent neutron scattering lengths to give S(q,$\omega$). To obtain S($\omega$), the resulting S(q,$\omega$) was integrated over the same q-window as accessible in experiment. To be specific, in order to conserve momentum and energy, the observable q-window in the experiment is

$$\frac{q^2\hbar^2}{2m_n} = 2E_i - \hbar\omega - 2\sqrt{(E_i - \hbar\omega)}cos(2\theta)$$

where $m_n$ is the rest mass of the neutron, $E_i$ is the kinetic energy of the neutron, $\hbar\omega$ is the energy transfer during the neutron scattering event, and $\theta$ is the scattering angle limits, set by the detector coverage so that $10 < 2\theta < 110$.

## II. X-RAY DIFFRACTION

X-ray diffraction was performed on a PANalytical Empyrean XRD using Cu $K_\alpha$ radiation ($\lambda = 1.547$ Å ) at ambient conditions. The data for the aluminium nanoparticles is shown in Fig. 2 a. Scherrer analysis (shown in inset) of the peak-broadening at the 111 Bragg reflection indicates an average particle size in reasonable agreement with those determined from TEM. The data for the $\gamma$ alumina is shown in Fig. 2 b. The very broad peaks indicates that the $\gamma$-phase particles consist of very small crystallites, on average, less than 5 nm in radius.

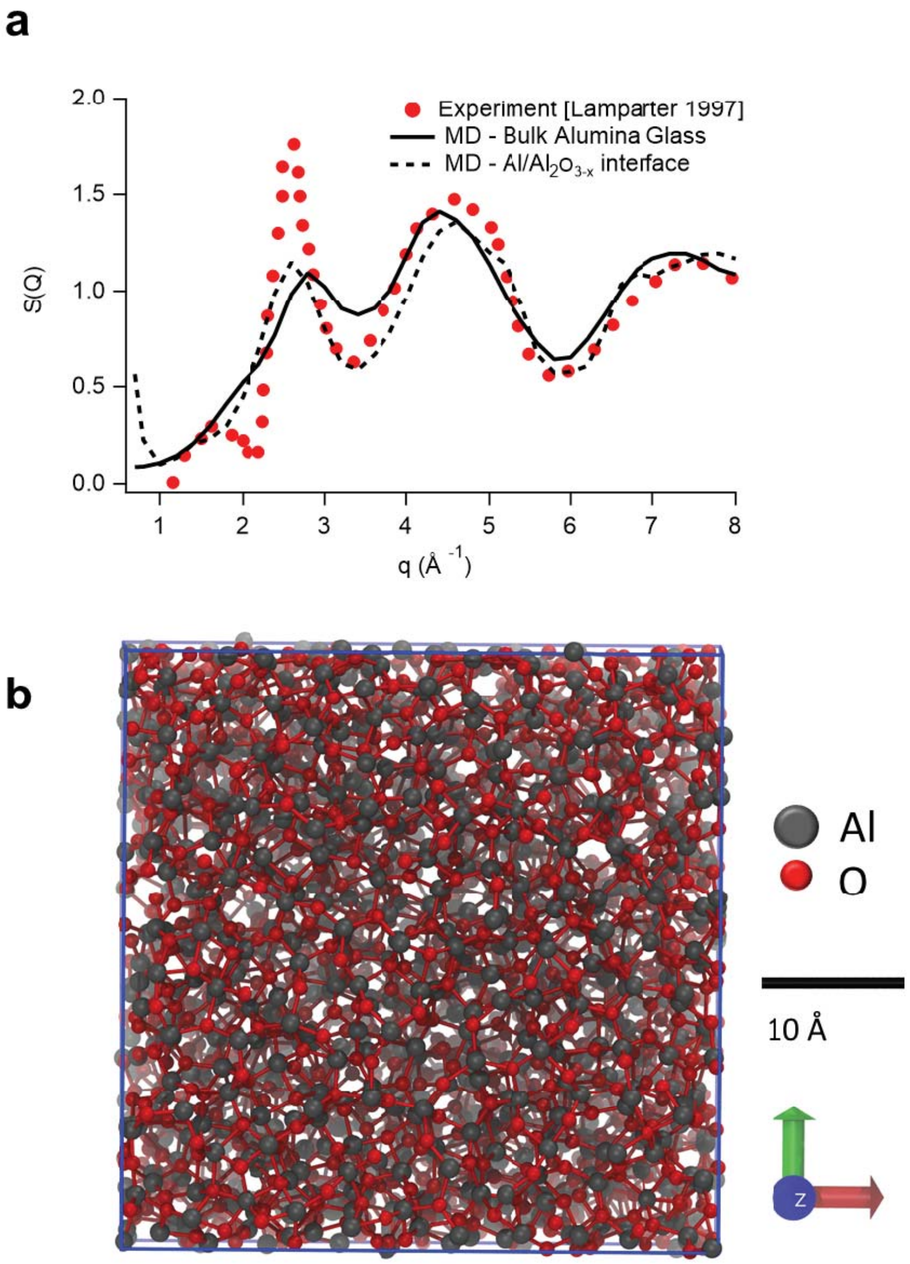


FIG. 1. a) Neutron static structure factor calculated by molecular dynamics for a bulk $Al_2O_3$ and the $Al/Al_2O_{3-x}$ interface, compared with previously published experimental data of anodised aluminium foils. [1]. b) Snapshot of the molecular dynamics trajectory of the bulk alumina glass.

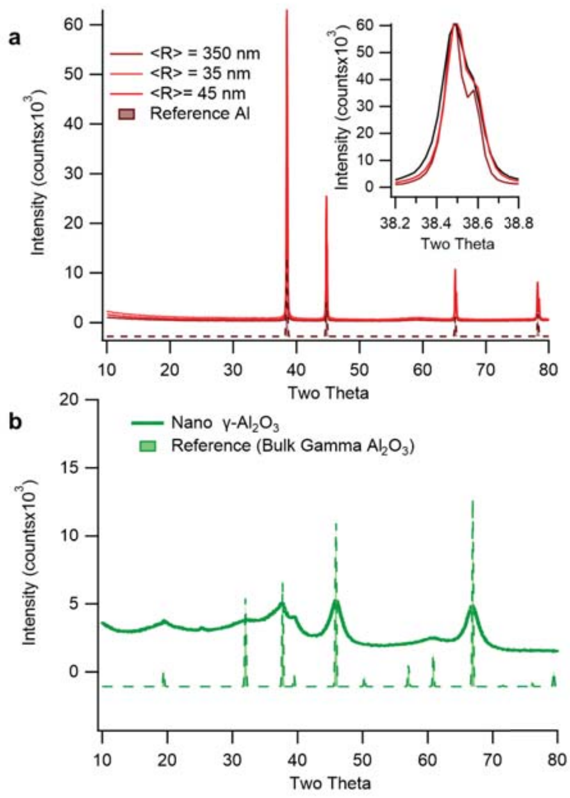


FIG. 2. a) The x-ray diffraction patterns for the various aluminium nanopowders are very similar and are dominated by crystalline aluminium Bragg peaks as shown by comparing to reference data for bulk Al. The inset shows an enlarged region of the (111) peak showing evidence of the Scherrer-broadening in the small particles. b) The X-ray diffraction pattern for the $\gamma$-phase alumina shows broad diffuse peaks consistent with a small particle size.

## III. TRANSMISSION ELECTRON MICROSCOPY

Transmission electron microscopy was performed on a JEOL2010 operating at 200 kV. The nanopowders were dispersed in ethanol and imaged on a lacy carbon grid. Figure a-c) 3 are bright field images comparing the microstructure of the metallic, corundum and $\gamma$ phase particles respectively.

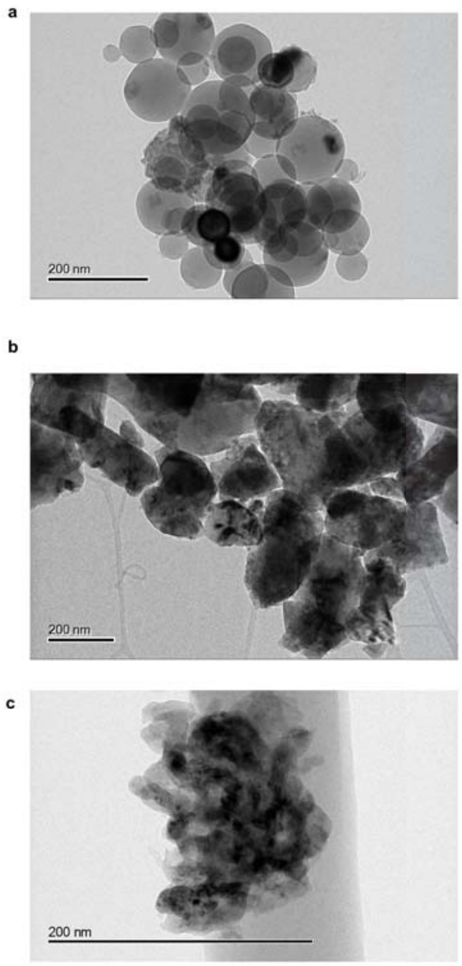


FIG. 3. a) TEM BF image for the <R>=35 nm aluminium nanopowder b) BF image for the $\alpha$ $Al_2O_3$nanopowder c) BF image for the $\gamma$ $Al_2O_{3-x}$ nanopowder showing presence of many small particles.

### A. Abberation-corrected TEM and Electron Energy Loss Spectroscopy

Abberation-corrected scanning transmission electron microscopy (STEM) was performed on a JEOL 200F operating at 200 keV, based at the Electron Microscopy Centre at the University of Wollongong. High-Angle, Annular Dark Field (HAADF) and bright-field images were obtained at atomic-scale resolution, together with electron energy loss spectroscopy (EELS). Figure 4 compares the HAADF and BF image of the Al/AlO interface of the aluminium nanoparticles, showing the amorphous nature of the oxide region. The EELS spectra were collected by mapping an interfacial region as shown in Figure 5 a. The spectra in the

a

b

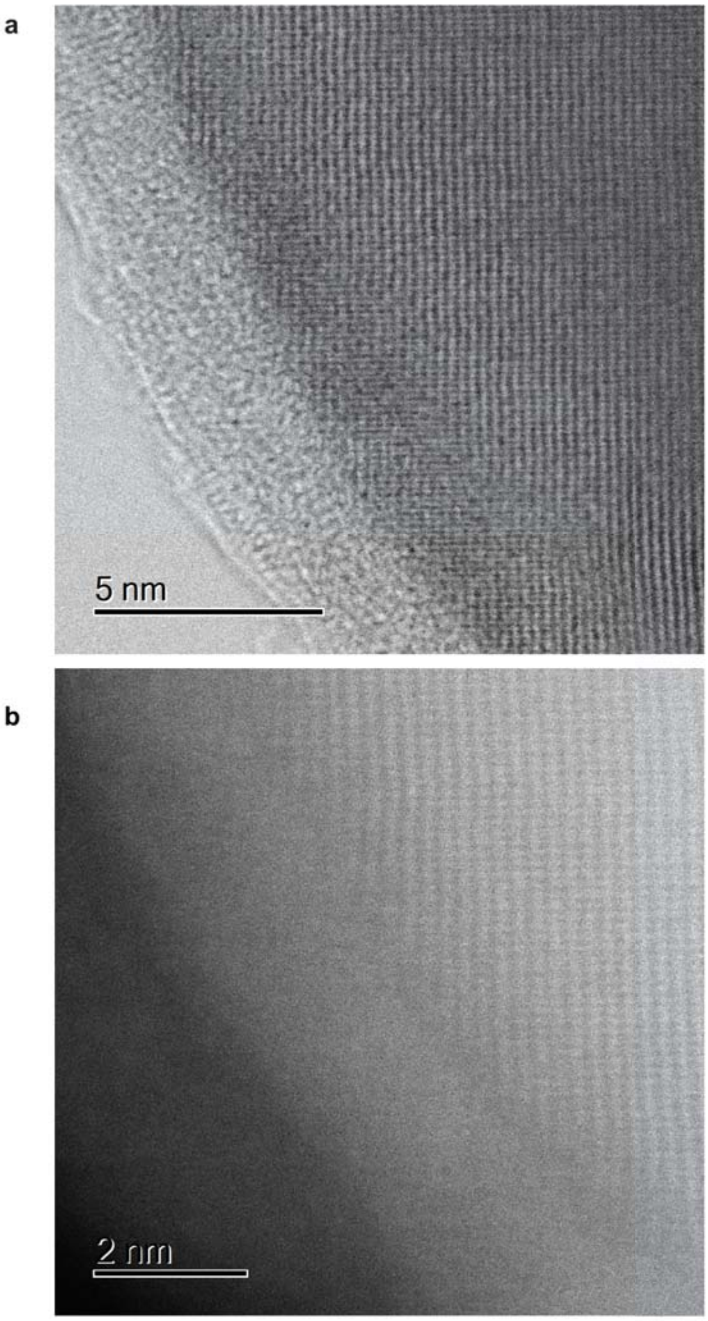


FIG. 4. a) BF image of the Al/$Al_2O_{3-x}$ interface b) HAADF image of the Al/$Al_2O_{3-x}$ interface

core of the aluminium particle are very similar to previously published EELS spectra for aluminium metal [6] as shown in Fig. 5 b. The spectra for the oxide shell region indicate a predominantly amorphous environment, as certain features differentiate this from the EELS in the crystalline $\gamma$ phase as shown in Fig. 5 c.

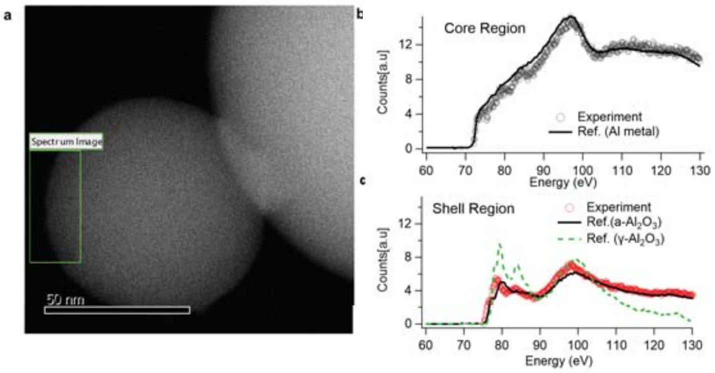


FIG. 5. a) Low magnification HAADF image of the aluminium nanoparticles showing the region studied using EELS b) EELS spectra for the Al core region c) EELS spectra for the oxide shell region compared with Reference data from Ref. 6.

## IV. REFERENCES


[1] P. Lamparter and R. Kniep, Physica B: Condensed Matter **234-236**, 405 (1997), proceedings of the First European Conference on Neutron Scattering.

[2] J. D. Gale, J. Chem. Soc., Faraday Trans. **93**, 629 (1997).

[3] W. G. Hoover, Phys. Rev. A **31**, 1695 (1985).

[4] W. Humphrey, A. Dalke, and K. Schulten, Journal of Molecular Graphics **14**, 33 (1996).

[5] K. Hinsen, E. Pellegrini, S. Stachura, and G. R. Kneller, J. Comp. Chem. **33**, 2043 (2012).

[6] D. Bouchet and C. Colliex, Ultramicroscopy **96**, 139 (2003).
